# Supplementary material for: Tracking the Takes and Trajectories of English-Language News Narratives across Trustworthy and Worrisome Websites
Source: arXiv:2501.09102 source file (2025-01-15)
Supplement: Supplementary file 1 [file appendix-stances.tex]

\section{Additional Stances\label{sec:additional-stances}}

\begin{figure}[!ht]
  \centering
  \includegraphics[width=1.0\columnwidth]{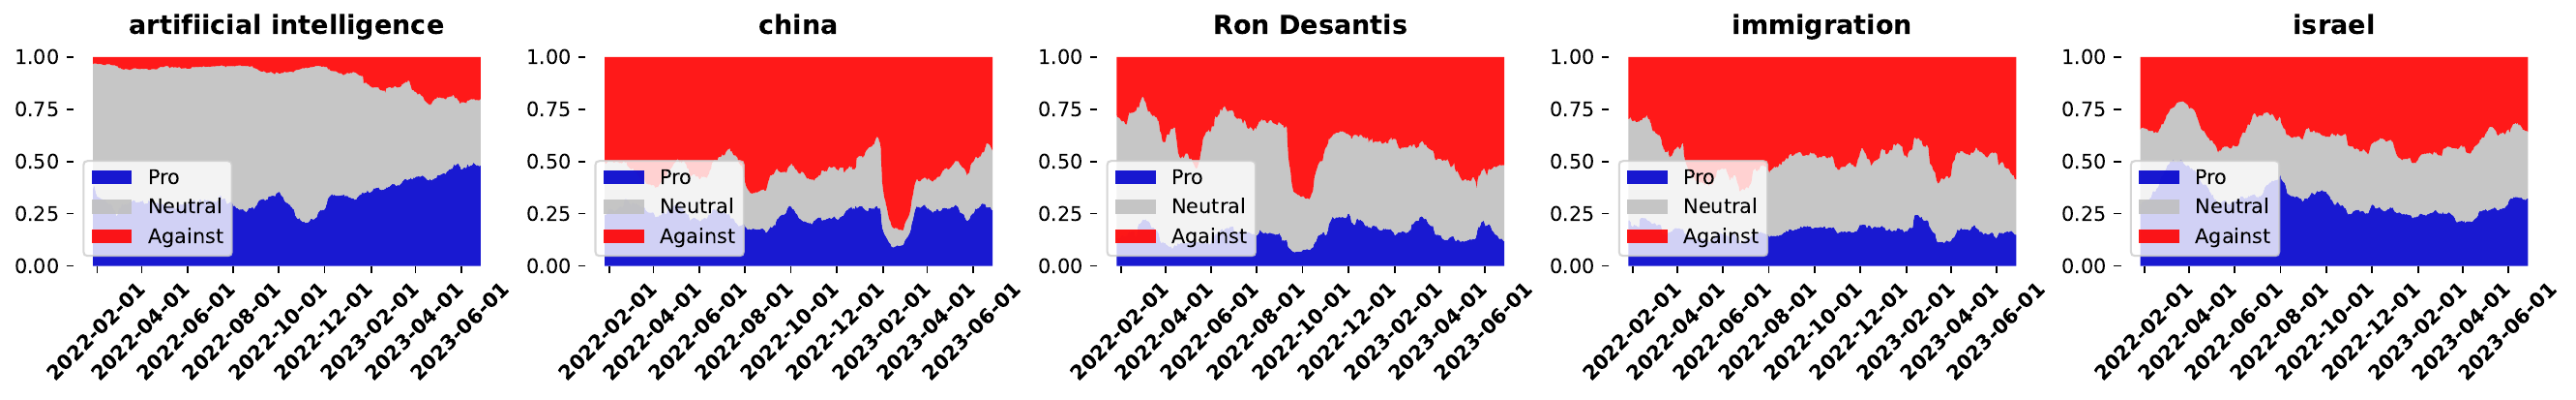}

\vspace{1pt}
\caption{Stance of authentic news websites to various popular entities over time. }
\label{fig:appendix-authentic-stance}
\end{figure}

\begin{table}[!ht]
\begin{minipage}{.22\textwidth}
\centering
%\scriptsize
\fontsize{5.5pt}{1pt}
\setlength{\tabcolsep}{1pt}
\selectfont
\begin{tabular}{ll}
\multicolumn{2}{c}{\textbf{Artificial Intelligence}} \\
\toprule
Pro Domains & Against Domains  \\ \midrule
nextbigfuture.com (72.1\%)  &futurism.com (52.4\%) \\
wdbj7.com (69.7\%) &vice.com (46.2\%) \\
kold.com (69.7\%) &commondreams.org (44.8\%)\\
\bottomrule
\end{tabular}
\end{minipage}
\begin{minipage}{.22\textwidth}
\centering
%\scriptsize
\fontsize{5.0pt}{1pt}
\setlength{\tabcolsep}{1pt}
\selectfont
\begin{tabular}{ll}
\multicolumn{2}{c}{\textbf{China}} \\
\toprule
Pro Domains & Against Domains  \\ \midrule
prnewswire.com (84.8\%) &defenseone.com (91.2\%) \\
cleantechnica.com (60.3\%)&conservativeinstitute.or (91.2\%) \\
frontiersin.org (59.6\%) & gizmodo.com (90.5\%)\\
\bottomrule
\end{tabular}
\end{minipage}
\begin{minipage}{.22\textwidth}
\centering
%\scriptsize
\fontsize{5.0pt}{1pt}
\setlength{\tabcolsep}{1pt}
\selectfont
\begin{tabular}{ll}
\multicolumn{2}{c}{\textbf{Ron Desantis}} \\
\toprule
Pro Domains & Against Domains  \\ \midrule
conservativeinstitute.org (48.6\%) &techdirt.com (83.7\%) \\
rasmussenreports.com (41.9\%)&abovethelaw.com (80.0\%) \\
christiannewsalerts.com (41.5\%) & queerty.com (79.4\%)\\
\bottomrule
\end{tabular}
\end{minipage}
\begin{minipage}{.22\textwidth}
\centering
%\scriptsize
\fontsize{5.0pt}{1pt}
\setlength{\tabcolsep}{1pt}
\selectfont
\begin{tabular}{ll}
\multicolumn{2}{c}{\textbf{Immigration}} \\
\toprule
Pro Domains & Against Domains  \\ \midrule
migrationpolicy.org (73.5\%) &channel4.com (96.4\%) \\
americanimmigrationcouncil.org (65.5\%)& bylinetimes.com (95.5\%) \\
mothership.sg (55.9\%) & leftfootforward.org (94.9\%)\\
\bottomrule
\end{tabular}
\end{minipage}
\begin{minipage}{.22\textwidth}
\centering
%\scriptsize
\fontsize{5.0pt}{1pt}
\setlength{\tabcolsep}{1pt}
\selectfont
\begin{tabular}{ll}
\multicolumn{2}{c}{\textbf{Israel}} \\
\toprule
Pro Domains & Against Domains  \\ \midrule
insidephilanthropy.com (100.0\%) &imeu.org (100.0\%) \\
israel21c.org (84.9\%)& freedomnews.org.uk (94.3\%) \\
defensenews.com (83.3\%) & freepress.org (93.0\%)\\
\bottomrule
\end{tabular}

\end{minipage}
\caption{The set of authentic news websites with the highest percentage of  \textit{Pro} and \textit{Against} articles about various entities/topics.}

\end{table}

\begin{figure*}[!htbp]
 \begin{subfigure}[b]{0.24\textwidth}
        \centering
        \includegraphics[width=\textwidth]{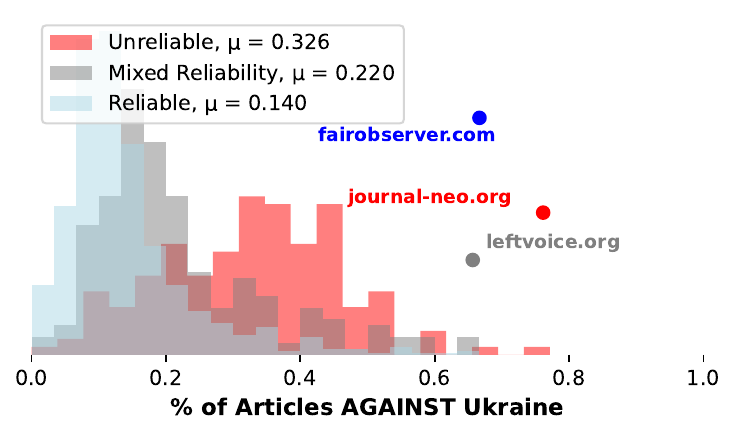}
        \caption{Dist. of Against Ukraine Articles}
        \label{fig:dist-against-ukraine}
    \end{subfigure}
    \begin{subfigure}[b]{0.24\textwidth}
        \centering
        \includegraphics[width=\textwidth]{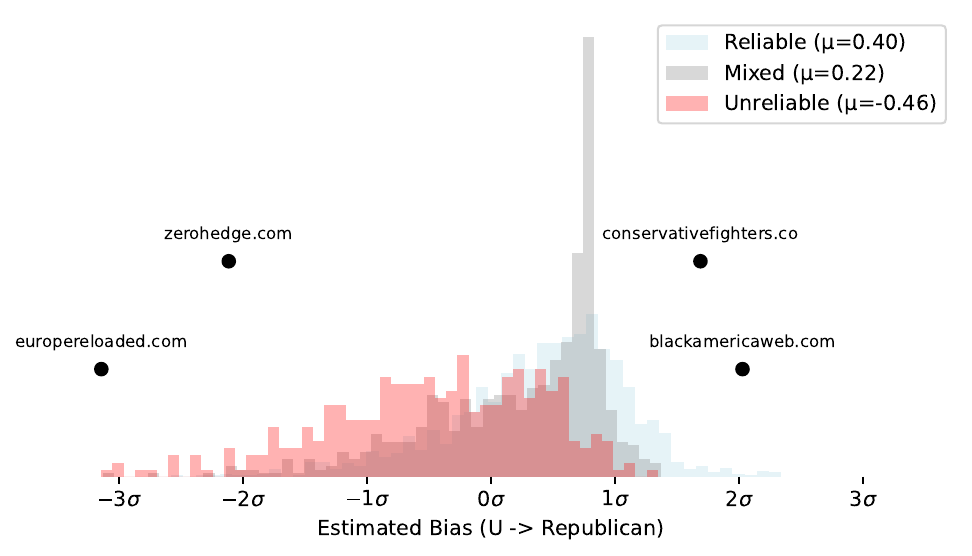}
        \caption{Ukraine Latent}
        \label{fig:ukraine-latent-dist}
    \end{subfigure}
    \begin{subfigure}[b]{0.24\textwidth}
        \centering
        \includegraphics[width=\textwidth]{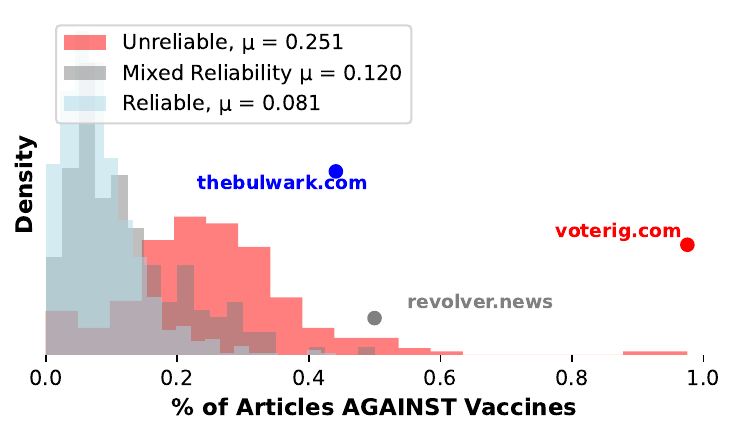}
        \caption{Dist. of Against Vaccines Articles}
        \label{fig:vaccine-against-dist}
    \end{subfigure}
 \centering
    \begin{subfigure}[b]{0.24\textwidth}
        \centering
        \includegraphics[width=\textwidth]{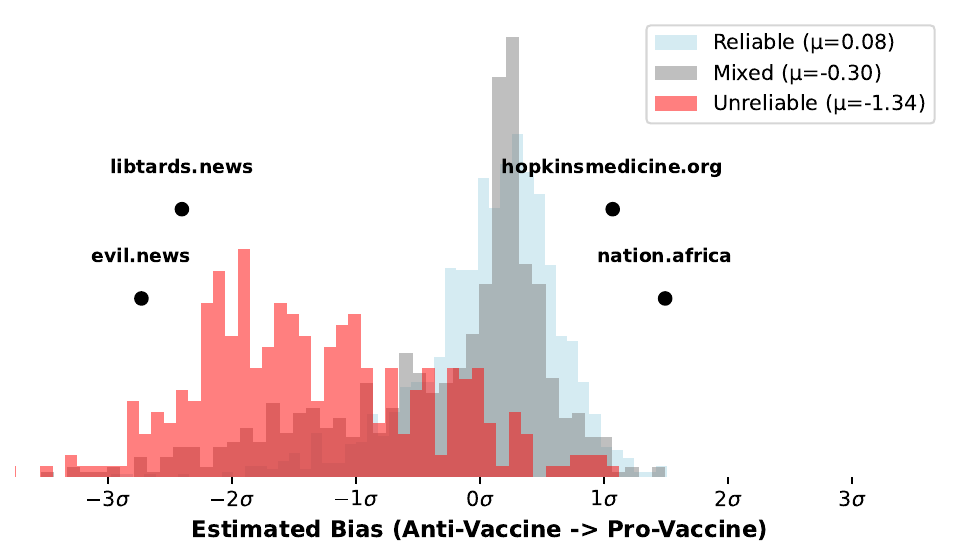}
        \caption{Vaccine Latent}
        \label{fig:vaccine-latent}
    \end{subfigure}

    \caption{Distribution of articles against various entities.}
    \label{fig:various-entities-dist}
\end{figure*}
